# Supplementary material for: SkyLogic - A proposal for a skyrmion logic device
Source: arXiv:1811.02016 source file (2018-11-05)
Supplement: Supplementary file 1 [file appendix.tex]

\begin{appendices}
%%%%%%%%%%%%%%%%%%%%%%%%%%%%%%%%%%%%%%%%%%%%%%%%%%%%%%%%%%%%%%%%%%%%%%%%%%%%%
\section{Derivation of skyrmion position equations}
\label{sec:appendixR2}

In this section, we first derive Equations~\eqref{eq:R2XDisp}
and~\eqref{eq:R2YDisp} from Equation~\eqref{eq:ThieleRegion1}. Next, we
show that Equations~\eqref{eq:R1XDisp} and~\eqref{eq:R1YDisp} can be
similarly be derived. Equation~\eqref{eq:ThieleRegion1}
can be written in the matrix notation as
\begin{equation}
	\begin{aligned}
		\begin{bmatrix}
			-Gv_{y,R2} \\
			 Gv_{x,R2}
		\end{bmatrix}
		+ \alpha 
		\begin{bmatrix}
			D & 0 \\
			0 & D
		\end{bmatrix}
		\begin{bmatrix}
			v_{x,R2} \\
			v_{y,R2}
		\end{bmatrix} = 
		\begin{bmatrix}
			F_{SHE,x} \\
			F_{SHE,y}
		\end{bmatrix} +
		\begin{bmatrix}
			0 \\
			F_{c,y}
		\end{bmatrix}.
	\label{eq:ThieleR2Matrix}
	\end{aligned}
\end{equation}
Equation~\eqref{eq:ThieleR2Matrix} can be written as a system of linear
equations as follows:
\begin{align*}
		-Gv_{y,R2} + \alpha D v_{x,R2} &= F_{SHE,x} \numberthis
\label{eq:ThieleR2SOE1} \\
		Gv_{x,R2}  + \alpha D v_{y,R2} &= F_{c,y} + F_{SHE,y}	\numberthis
\label{eq:ThieleR2SOE2}.
\end{align*}	
Solving Equations~\eqref{eq:ThieleR2SOE1} and~\eqref{eq:ThieleR2SOE2} and
substituting $F_{c,y} = -k y_{R2}(t)$, we obtain $v_{x,R2}$ and $v_{y,R2}$ as 
\begin{align*}
	v_{x,R2} &= \frac{dx_{R2}(t)}{dt} = AF_{SHE,x} + B(F_{SHE,y}
-ky_{R2}(t)) \numberthis \label{eq:Thiele2vx} \\
	v_{y,R2} &=  \frac{dy_{R2}(t)}{dt} = -BF_{SHE,x} +A(F_{SHE,y} -
ky_{R2}(t)) \numberthis \label{eq:Thiele2vy}
\end{align*}
where 
\begin{equation}
	A = \frac{\alpha D}{G^2+(\alpha D)^2} ; B = \frac{G}{G^2+(\alpha
D)^2}.
\label{eq:ABconst}
\end{equation}
\noindent
Integrating Equation~\eqref{eq:Thiele2vx} over time with the initial
conditions, $x_{R2}(t=0) = x_{R2}(t_0)$ and $y_{R2}(t=0) = y_{R2}(t_0)$, and
using the relation in Equation~\eqref{eq:tau}, we obtain $x_{R2}(t)$ in
the form of Equation~\eqref{eq:R2XDisp} as
\begin{align*}
	x_{R2}(t) =& \; \; x_{R1}(t_0) + \\
& \Bigg(\frac{t}{\tau}\Bigg)\Bigg[\frac{F_{SHE,x}}{k} +
\frac{GF_{SHE,y}}{\alpha D k} - 
\frac{G}{\alpha D} y_{R2}(t) \Bigg] \numberthis \label{eq:R2XDispApx}.
\end{align*}
Equation~\eqref{eq:Thiele2vy} is a first-order differential equation of the form
\begin{equation}
	\frac{df(t)}{dt} = P_1 + P_2 f(t),
\label{eq:diffEq}
\end{equation}
\noindent
whose solution is given by
\begin{equation}
	f(t) = \frac{-P_1}{P_2} +
\Bigg(f(t_0)+\frac{P_1}{P_2}\Bigg)e^{P_2t}
	\label{eq:diffEqSoln}
\end{equation}
Here $f(t)$, $f(t_0)$, $P_1$, and $P_2$ are given by 
\begin{align*}
f(t) &= y_{R2}(t); & 
		f(t_0) &= y_{R2}(t_0);  \numberthis \label{eq:P1P2const} \\ 
P_1 &= -BF_{SHE,x}+AF_{SHE,y}; &
		P_2 &= -Ak = -\frac{1}{\tau}.
\end{align*}
Substituting $f(t)$, $P_1$, and $P_2$ from Equation~\eqref{eq:P1P2const} and
$f(t_0) = y_{R2}(t_1)$ in Equation~\eqref{eq:diffEqSoln} we obtain $y_{R2}(t)$
in the form of Equation~\eqref{eq:R2YDisp} as
\begin{align*}
	y_{R2}(t) =& \; \; y_{R2}(t_1)e^{-t/\tau } + \\
& \Bigg[\frac{G F_{SHE,x}}{\alpha D k} -
\frac{F_{SHE,y}}{k}\Bigg]\Big(e^{-t/\tau} - 1 \Big) 
\end{align*}

Equations~\eqref{eq:R1XDisp} and \eqref{eq:R1YDisp} can be similarly derived
from Equations~\eqref{eq:ThieleR2SOE1} and ~\eqref{eq:ThieleR2SOE2} by setting
$F_{SHE,y} = 0$ and replacing $v_{x,R2}$ and $v_{y,R2}$ by $v_{x,R1}$ and
$v_{y,R1}$, respectively.   
\end{appendices}
